# Supplementary material for: Spatio-temporal topology of plasmonic spin meron pairs revealed by polarimetric photo-emission microscopy
Source: arXiv:2411.03262 source file (2024-11-06)
Supplement: Supplementary file 1 [file Supplementary_Material.pdf]

**Spatio-temporal topology of plasmonic vector fields revealed by polarimetric photoemission microscopy**

Pascal Dreher[1], Alexander Neuhaus[1], David Janoschka[1], Alexandra Rödl[1], Tim Meiler[2], Bettina Frank[2], Timothy J. Davis[1,2,3*], Harald Giessen[2*], and Frank-J. Meyer zu Heringdorf[1*]

[1] Faculty of Physics and Center for Nanointegration, Duisburg-Essen (CENIDE), University of Duisburg-Essen, 47048 Duisburg, Germany

[2] 4th Physics Institute, Research Center SCoPE, and Integrated Quantum Science and Technology Center, University of Stuttgart, 70569 Stuttgart, Germany

[3] School of Physics, University of Melbourne, Parkville Victoria 3010 Australia

*Correspondence to: timd@unimelb.edu.au (T.D.); meyerzh@uni-due.de (F.-J.M.z.H.); giessen@pi4.uni-stuttgart.de (H.G.)

**Supplementary Note 1:** Interferometer for Polarimetry

Pump-probe pulses for the time-resolved polarimetry experiments are generated by a home-built Mach-Zehnder interferometer that is actively phase-stabilized using Pancharatnam's phase [1]. The optical setup of the interferometer is depicted in Supplementary Fig. 1. Adjusting the polarizations of the femtosecond pump- and probe pulses is accomplished by half-waveplates in each of the two arms of the interferometer, $\lambda_{1/2}^{\text{pump}}$ and $\lambda_{1/2}^{\text{probe}}$. As the beam splitters in the interferometer and subsequent mirrors within the optical setup modify the polarization states, a combination of half- and quarter waveplate has been added to the output of the interferometer. Each of the pump- and probe-pulses thus passes through three (motorized) waveplates:

$$\text{Pump Pulses: } \lambda_{1/2}^{\text{pump}}, \lambda_{1/2}^{(\text{O})}, \lambda_{1/4}^{(\text{O})} \qquad \text{and} \qquad \text{Probe Pulses: } \lambda_{1/2}^{\text{probe}}, \lambda_{1/2}^{(\text{O})}, \lambda_{1/4}^{(\text{O})}$$

whereas both pump and probe pulses pass through the same $\lambda_{1/2}^{(\text{O})}$ and $\lambda_{1/4}^{(\text{O})}$ waveplates. Any polarization state can be selected for the pump, whereas the attainable probe polarizations for a given pump polarization are somewhat limited. Furthermore, the differently polarized probe pulses should exhibit somewhat similar intensity. All polarization states are verified by measuring their Stokes vector with a commercial polarimeter placed in a conjugate sample plane. Usually, to actively stabilize the interferometer, linearly polarized HeNe laser beams of orthogonal polarization are passed through the interferometer, and the intensity of the HeNe interference signal at the output of the interferometer is measured with a photodiode behind a $\lambda_{1/4}^{\text{HeNe}}$ waveplate and a polarizer [1,2]. Rotating the polarizer causes the intensity on the diode to change, which is the input signal for a home-built proportional-integral-differential (PID) feedback loop that moves the piezo-driven delay stage. In this way the interferometer is actively stabilized, and the delay can be adjusted by rotating the polarizer. Unfortunately, inserting motorized polarization optics into the two arms of the interferometer also affects the HeNe laser polarization and thus affects the Pancharatnam's phase stabilization concept. To circumvent this problem, we added $\lambda_{1/4}^{\text{HeNe}}$ quarter-waveplates to each of the arms of the interferometer so that only the HeNe beams passed through them. The achromatic pump-probe polarization waveplates $\lambda_{1/2}^{\text{pump}}$ and $\lambda_{1/2}^{\text{probe}}$ then only introduce a phase-shift into the HeNe beam. To avoid destruction of the circular polarization of the HeNe beam by subsequent optics, the HeNe polarizations in the two arms are converted back to linear (and orthogonal) polarization by two thin-film polarizers. Again, these polarizers are mounted so that only the HeNe beams pass through them. In this configuration a change of the pump- or probe polarization does not affect the intensity, the linear polarization state of the HeNe beams, or the working principle of the stabilization. Instead, a change in pump-probe polarization merely introduces a phase shift in the HeNe signal. The feedback loop of the stabilization responds to the phase shift and transfers it over to a shift of the temporal

overlap of the femtosecond laser pulses. A solution to this problem will be discussed in Supplementary Note 2.

To estimate the temporal resolution, we have extensively investigated the long-term stability as well as the temporal jitter of the stabilized interferometer. Performing a pump-probe experiment with the presented interferometer on a single groove we monitored the position of a (plane-wave) SPP wave-packet over several hours using the fastest sampling rate of our detector (200 ms exposures) to characterize the *in-situ* temporal stability. Using this method, we could verify temporal jitters to be well-below 100 attoseconds and could not find any long-term temporal drift. We conclude that our temporal resolution is well-below the delay scanning step size, which is thus the fundamental limit for the temporal resolution.

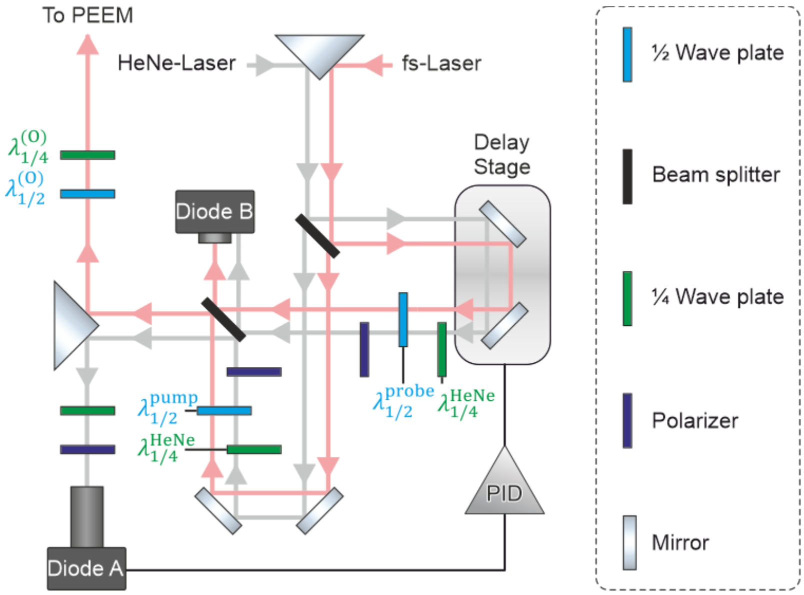


**Supplementary Figure 1:** Overview of the optical setup of the interferometer used for polarimetry. A HeNe laser beam (grey) is passed in parallel to the fs pulses (light red) through a phase-stabilized Mach-Zehnder interferometer. The polarization state of the fs pump- and probe pulses can be adjusted using the four waveplates $\lambda_{1/2}^{\text{pump}}$, $\lambda_{1/2}^{\text{probe}}$, $\lambda_{1/2}^{(O)}$ and $\lambda_{1/4}^{(O)}$. The combination of the two quarter waveplates $\lambda_{1/4}^{\text{HeNe}}$ with subsequent polarizers ensures that the phase-stabilization works for all possible pump- and probe polarizations.

**Supplementary Note 2:** Delay Time Correction and Phase Extraction

A rotation of the $\lambda_{1/2}^{\text{probe}}$ waveplate introduces a phase-shift into the HeNe section of the interferometer which changes the HeNe signal on Diode A in Supplementary Fig. 1 and which in turn causes the stabilization to change the delay stage position in the interferometer. As such, pump-probe images taken at the same *nominal* delay but with different probe polarizations will represent the situation at different delay times. A precise determination of the time-zero condition for every polarization is crucial for a successful polarimetric vector-field reconstruction. At every nominal delay step and for every polarization state of the experiment, the laser is switched with a motorized flip-mirror between the PEEM and an optical spectrometer, where the linear interference of pump- and probe pulses (spectral interference) is measured. The spectral interference measurements recorded during the meron pair experiment are shown as function of delay time for the four used probe polarizations in Supplementary Fig. 2.

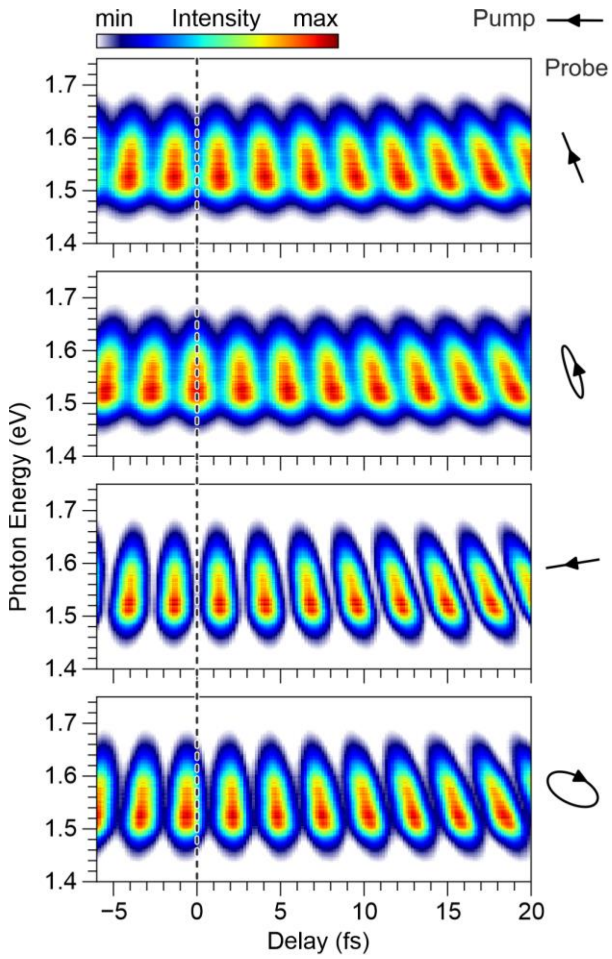


**Supplementary Figure 2:** Spectral interference. The output of the interferometer is directed to an optical spectrometer and spectrally resolved autocorrelation traces are recorded. A two-dimensional fit to the data using a plane-wave model provides the true point of zero-time delay.

For all polarizations and at all photon energies a periodic arrangement of maxima and minima in the spectral interference is clearly visible. This oscillation resembles the interference at different wavelength components comprising the fs laser pulses. As higher photon energies correspond to shorter oscillation periods, the maxima are inclined, and the inclination increases with delay time. As such, only at the time of exact temporal overlap (time zero, $\Delta t = 0$ fs) the inclination would be absent.

Only the Stokes vectors of the pump and probe polarizations are accessible to a polarimetric measurement, while the full-phased Jones vectors are needed for the reconstruction of the polarimetric PEEM data. Unfortunately, there is no bijective mapping between Stokes and Jones vectors, since the Jones vectors can always contain an additional phase that is not included in the Stokes vectors.

Both the time zero and the phase difference between the Jones vectors of the pump and probe pulses can be extracted from the spectral interference in Supplementary Fig. 2. For every polarization the spectral interference is numerically fitted by a simple plane wave model, containing the time-zero, the phase difference of the pump- and probe Jones vectors, and a calibration of the actual delay time as fit parameters. Note that the data in Supplementary Fig. 2 has already been horizontally shifted so that the time zero is the same for all polarization series.

**Supplementary Note 3:** PEEM Data Analysis Pipeline

Pump-probe sequences with different probe polarization are fed into a standardized data analysis pipeline that is similar to the one we have used in earlier work [3]. In a perfect experiment, two (mostly orthogonal) probe polarizations would be sufficient for a complete characterization of the components of the SPP field in the surface plane. As the pump polarization must be adjusted to match the requirements of the SPP excitation structure, however, adequate probe polarizations cannot always be achieved. Instead, we sample the SPP field using several different probe polarizations that roughly cover the Poincaré sphere. The loosened requirement for the probe polarizations is ultimately an advantage of our method since we do not need to precisely control the probe polarization but merely need to precisely measure it. This approach is similar to standard polarimetric imaging in optics or phase-front estimations using interferograms (see for example Supplementary Ref. [4]), where multiple redundant measurements provide an overdetermined system and are used to tremendously reduce measurement errors. In our current work, using four different probe polarizations has proven to be a good compromise between measurement time and fulfilling the above requirements.

The four raw PEEM images in Supplementary Fig. 3a were recorded at identical pump but different probe polarizations and thus show different probing of the same SPP field. Clearly, the different relative polarizations manifest themselves in the angular distribution of the PEEM signal. As a first step of the data analysis the individual images in each polarization sequence are drift-corrected using standard cross-correlation drift techniques. Afterwards, we extract a signal from the data that corresponds to the scalar product between SPP field vector and probe field vector as follows: In a normal-incidence geometry, the SPP related and delay time $\Delta t$ dependent local yield $Y_{\mathrm{2PPE}}(\mathbf{r}, \Delta t)$ in the nonlinear PEEM images far away from the exciting Archimedean spiral is determined by [5] $Y_{\mathrm{2PPE}}(\mathbf{r}, \Delta t) = \int_{-\infty}^{\infty} \left| \mathbf{E}_{\mathrm{probe}}(t - \Delta t) + \mathbf{E}_{\mathrm{spp}}(\mathbf{r}, t) \right|^4 \mathrm{d}t$. Here, $\mathbf{E}_{\mathrm{spp}}(\mathbf{r}, t)$ describes the spatially varying SPP field and $\mathbf{E}_{\mathrm{probe}}(t - \Delta t)$ represents the time-delayed but spatially homogeneous probe laser pulse. Note that this equation can be easily converted into the representation given in Supplementary Ref. [3] by linearizing the expression in the SPP field.

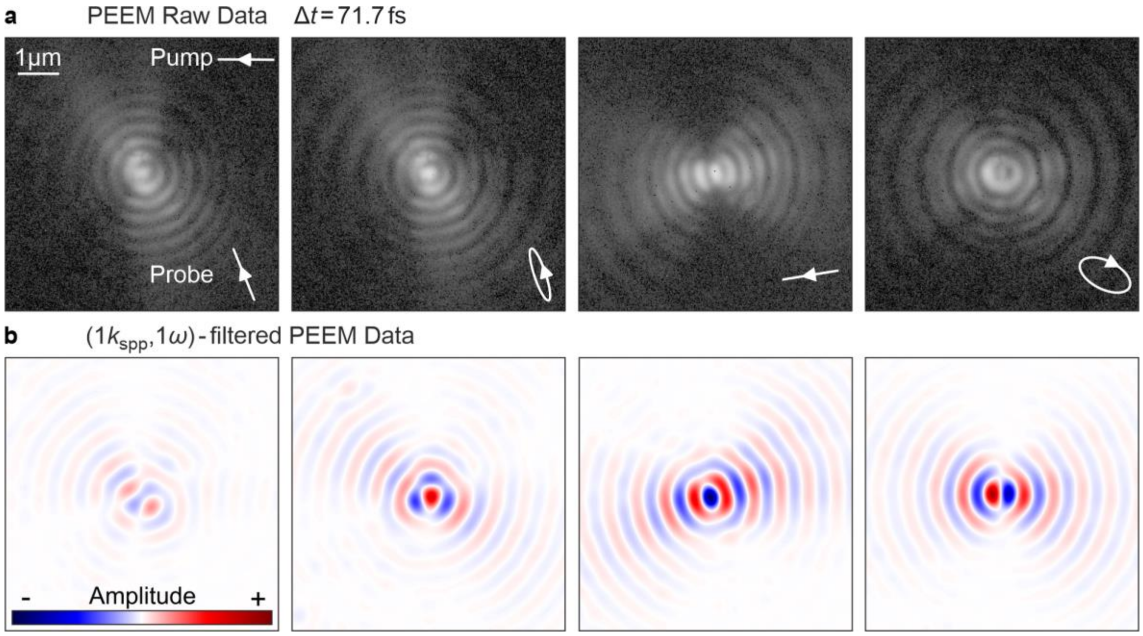


**Supplementary Figure 3:** (a) Raw PEEM data for linear pump and different probe polarizations on a logarithmic color scale and (b) the real part of the corresponding Fourier-filtered images in a linear false-color representation. In the raw data the signal is dominated by plasmoemission, which can be filtered out due to its dependence on the angular frequency $\omega$ and the wavevector $\mathbf{k}_{\mathrm{SPP}}$.

To emphasize the next step of the data processing, we neglect pulse envelopes and express the argument of the integral as an averaged emission rate. The expansion of the binomial results in

$$\begin{aligned}\bar{\Gamma}_{\mathrm{SPP}}(\mathbf{r}) \propto & \left|\mathbf{E}_{\mathrm{spp}}(\mathbf{r})\right|^4 + \left|\mathbf{E}_{\mathrm{probe}}\right|^4 + 4\left|\mathbf{E}_{\mathrm{probe}}\right|^2 \cdot \left|\mathbf{E}_{\mathrm{spp}}(\mathbf{r})\right|^2 \\ & +4\left(\left|\mathbf{E}_{\mathrm{probe}}\right|^2 + \left|\mathbf{E}_{\mathrm{spp}}(\mathbf{r})\right|^2\right) \cdot \operatorname{Re}\left\{\mathbf{E}^*_{\mathrm{probe}} \cdot \mathbf{E}_{\mathrm{spp}}(\mathbf{r}) \cdot \exp\left(i\left(\mathbf{k}_{\mathrm{spp}} \cdot \mathbf{r} - \omega\,\Delta t\right)\right)\right\} \\ & +2\operatorname{Re}\left\{\mathbf{E}^*_{\mathrm{probe}} \cdot \mathbf{E}_{\mathrm{spp}} \cdot \exp\left(i\left(2\,\mathbf{k}_{\mathrm{spp}} \cdot \mathbf{r} - 2\,\omega\,\Delta t\right)\right)\right\}.\end{aligned} \qquad \text{(Eq. 1)}$$

All terms of the above equation, however, contribute to the electron yield and the SPP-related signal of interest is superposed by static and delay time dependent contributions. It is important to note that only the argument of the exp(...) function in the fourth term depends directly on $1 \cdot \mathbf{k}_{\mathrm{spp}}$ and $1 \cdot \omega$, i.e., on the momentum vector and the angular frequency of the SPP. The nonlinear mixing of fields in different power is understood by quantum path interferences [6] and it is the purpose of the following data analysis to extract $\mathbf{E}_{\mathrm{spp}}$.

To separate the fourth term of the Supplementary Equation 1 from the raw data we first Fourier-filter the data spatio-temporally to the fundamental frequency $1 \cdot \omega$ and the SPP momentum $1 \cdot |\mathbf{k}_{\mathrm{spp}}|$. The temporal Fourier-filtering of our photoemission signal is performed such that only the positive-frequency part is maintained. Note that such filtering was already applied to the data in our earlier work [3] and that it has also been used in other topological PEEM work [7].

The real part of the Fourier-Filtered images of the upper panels in Supplementary Fig. 3a are shown as Supplementary Fig. 3b. The filtered data represents the complex projection of the SPP as excited by the pump-pulse on the different probe polarizations, with all other contributions to the PEEM signal filtered out. The relevant part of the emission rate is then proportional to

$$\Gamma_{1\omega,1\mathrm{k}}(\mathbf{r}) \propto \left(\left|\mathbf{E}_{\mathrm{probe}}\right|^2 + \left|\mathbf{E}_{\mathrm{spp}}(\mathbf{r})\right|^2\right)\left|\mathbf{E}_{\mathrm{probe}}\right| \mathbf{J} \cdot \mathbf{E}_{\mathrm{spp},\parallel},$$

where the probe electric field $\mathbf{E}_{\mathrm{probe}}$ is expressed by its magnitude $\left|\mathbf{E}_{\mathrm{probe}}\right|$ multiplied with the corresponding Jones vector $\mathbf{J}$ to describe the correctly phased polarization state. We divide the extracted signal by $\left|\mathbf{E}_{\mathrm{probe}}\right|^3$ for each probe polarization to normalize the yield to the part linear in $\mathbf{E}_{\mathrm{spp}}$. Furthermore, we combine the equations for all polarizations into one equation by introducing matrices $\underline{\mathbf{A}}$ and $\underline{\mathbf{M}}$. The extracted photoemission yield for all probe polarizations can be written for every time delay as a function containing the scalar SPP scaling factor β

$$\mathbf{Y}_{1\omega,1\mathrm{k}}(\mathbf{r}) = \left(\underline{\mathbf{1}} + \beta\underline{\mathbf{A}}\left|\mathbf{E}_{\mathrm{spp}}(\mathbf{r})\right|^2\right)\underline{\mathbf{M}}\,\mathbf{E}_{\mathrm{spp},\parallel}(\mathbf{r}). \qquad \text{(Eq. 2)}$$

Note that the respective contribution to the photoemission yield $\mathbf{Y}_{1\omega,1\mathrm{k}}(\mathbf{r})$ and all electric fields are complex numbers due to the Fourier-filtering. In the case of $n$ probe polarizations the diagonal $(n \times n)$ matrix contains the inverse probe intensities $\left|\mathbf{E}_{\mathrm{probe,i}}\right|^{-2}$

$$\underline{\mathbf{A}} = \begin{pmatrix} \left|\mathbf{E}_{\mathrm{probe},1}\right|^{-2} & \cdots & 0 \\ \vdots & \ddots & \vdots \\ 0 & \cdots & \left|\mathbf{E}_{\mathrm{probe},n}\right|^{-2} \end{pmatrix}.$$

The matrix $\underline{\mathbf{M}}$ in Supplementary Eq. 2 contains the complex 2D Jones vectors of all used probe polarizations, i.e., with $n$ probe polarizations $\underline{\mathbf{M}}$ becomes a $(n \times 2)$ matrix. Due to the normal incidence geometry, the electric field of the probe pulse lies within the surface plane and therefore $\underline{\mathbf{M}}$ only acts on the in-plane component of the SPP field $\mathbf{E}_{\mathrm{spp},\parallel}(\mathbf{r})$. A reconstruction of $\mathbf{E}_{\mathrm{spp}}(\mathbf{r})$ using Supplementary Eq. 2 then relies on the knowledge of the exact Jones vectors of all probe polarizations in relation to the Jones vector of the pump polarization. Unfortunately, only the Stokes vector of a polarization

states is accessible to a direct measurement, and the Jones vectors must be determined from a spectral interference measurement. This procedure is described in Supplementary Note 2.

With the knowledge of $\underline{\mathbf{M}}$, Supplementary Eq. 2 can be inverted to form a fixed-point equation for the SPP's electric field in the surface plane

$$\mathbf{E}_{\mathrm{spp},\parallel} = \underline{\mathbf{M}}^{-1}\left(\underline{\mathbf{1}} + \beta\underline{\mathbf{A}}\left|\mathbf{E}_{\mathrm{spp}}\right|^{2}\right)^{-1}\mathbf{Y}_{1\omega,1\mathrm{k}}(\mathbf{r}), \qquad \text{(Eq. 3)}$$

where $\underline{\mathbf{M}}^{-1}$ is the Moore-Penrose pseudo-inverse of $\underline{\mathbf{M}}$. It is important to emphasize that $\left|\mathbf{E}_{\mathrm{spp}}\right|^{2}$ also contains the component $\mathbf{E}_{\mathrm{spp},\perp}$ of the SPP field that is perpendicular to the surface plane. We use the divergence free nature of the continuous fields in the vacuum which, combined with the evanescent character of the SPP field in the direction perpendicular to the surface plane, allows to calculate $\mathbf{E}_{\mathrm{spp},\perp}$ from $\mathbf{E}_{\mathrm{spp},\parallel}$ using Maxwell's equations. To account for surface and volume effects in the photoemission process, we follow the work by Podbiel et al. [8] and introduce a scaling parameter $\alpha$ to balance the photoemission yields from $\mathbf{E}_{\mathrm{spp},\perp}$ and $\mathbf{E}_{\mathrm{spp},\parallel}$

$$\left|\mathbf{E}_{\mathrm{spp}}\right|^{2} \mapsto \left|\mathbf{E}_{\mathrm{spp},\parallel}\right|^{2} + \alpha\left|\mathbf{E}_{\mathrm{spp},\perp}\right|^{2}.$$

Supplementary Eq. 3 can then be solved by a numerical fixed-point iteration, and the scaling parameters $\alpha$ and $\beta$ are determined by minimizing the deviation between the experimental (and Fourier-filtered) yield and the yield calculated from the reconstructed fields. As a starting point for the fixed-point iteration, we assume no SPP fields on the surface. Note that the aforementioned calculation of $\mathbf{E}_{\mathrm{spp},\perp}$ from $\mathbf{E}_{\mathrm{spp},\parallel}$ has to be performed within each iteration. Using Maxwell's equation $\boldsymbol{\nabla} \times \mathbf{E}_{\mathrm{SPP}} = -\mu_0 \partial_t \mathbf{H}$ we can calculate the time-dependent magnetic field from the time-dependent electric SPP field, assuming that the envelope of the pulses is longer than the oscillation period.

**Supplementary Note 4:** Sample design

Details of the used excitation structures are shown in Supplementary Fig. 4a for a trimeron (discussed in Supplementary Note 5) and Supplementary Fig. 4b for the meron pair (discussed in the main document), respectively. Scanning electron microscopy (SEM) images of each structure are shown as greyscale images. The dark curved lines in the SEM images correspond to the FIB-milled grooves at which SPPs are excited. The dashed white circles mark discontinuities within the excitation structures with a gap-size of one SPP wavelength. The excitation structure for the trimeron in Supplementary Fig. 4a is a segmented Archimedean spiral with two gaps and a total orbital angular momentum of $l = 2$. The structure for the meron pair in Supplementary Fig. 4b is a simple non-segmented Archimedean spiral with only one gap and an orbital angular momentum of $l = 1$. The rendered images of the Au platelets illustrate the choice of pump-polarization relative to the gaps in the structure. In both cases the linear polarization direction was chosen to be orthogonal to a fictitious line through the endpoints of the gaps.

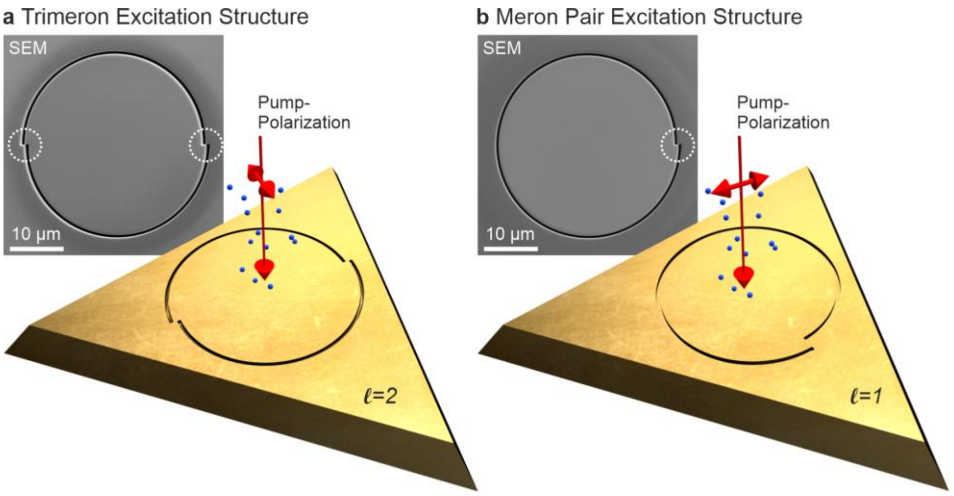


**Supplementary Figure 4:** The used excitation structures for (a) the trimeron and (b) the meron pair alongside illustrations of the used excitation polarization. The open red circles in the scanning electron microscopy (SEM) images indicate locations where the excitation grove of the spiral structure exhibits a gap of one SPP wavelength.

**Supplementary Note 5:** Analysis of a trimeron SAM texture for comparison with previous work

To benchmark our new polarimetric PEEM method, we analyzed an excitation structure like the one in Supplementary Fig. 4a to create a trimeron in the center of an Archimedean spiral with $l = 2$ that was excited with linearly polarized fs laser pulses. Such a trimeron has already been analyzed by Dai et al. [7], and the authors used an optical flow algorithm to extract the L-line topology from a time-resolved PEEM experiment. In our benchmark experiment, we performed a full determination of the electric, magnetic and SAM fields of the trimeron and determined the position of L-lines, the Chern density, and numerically integrated the Chern density over the L-line contour to obtain the Chern number.

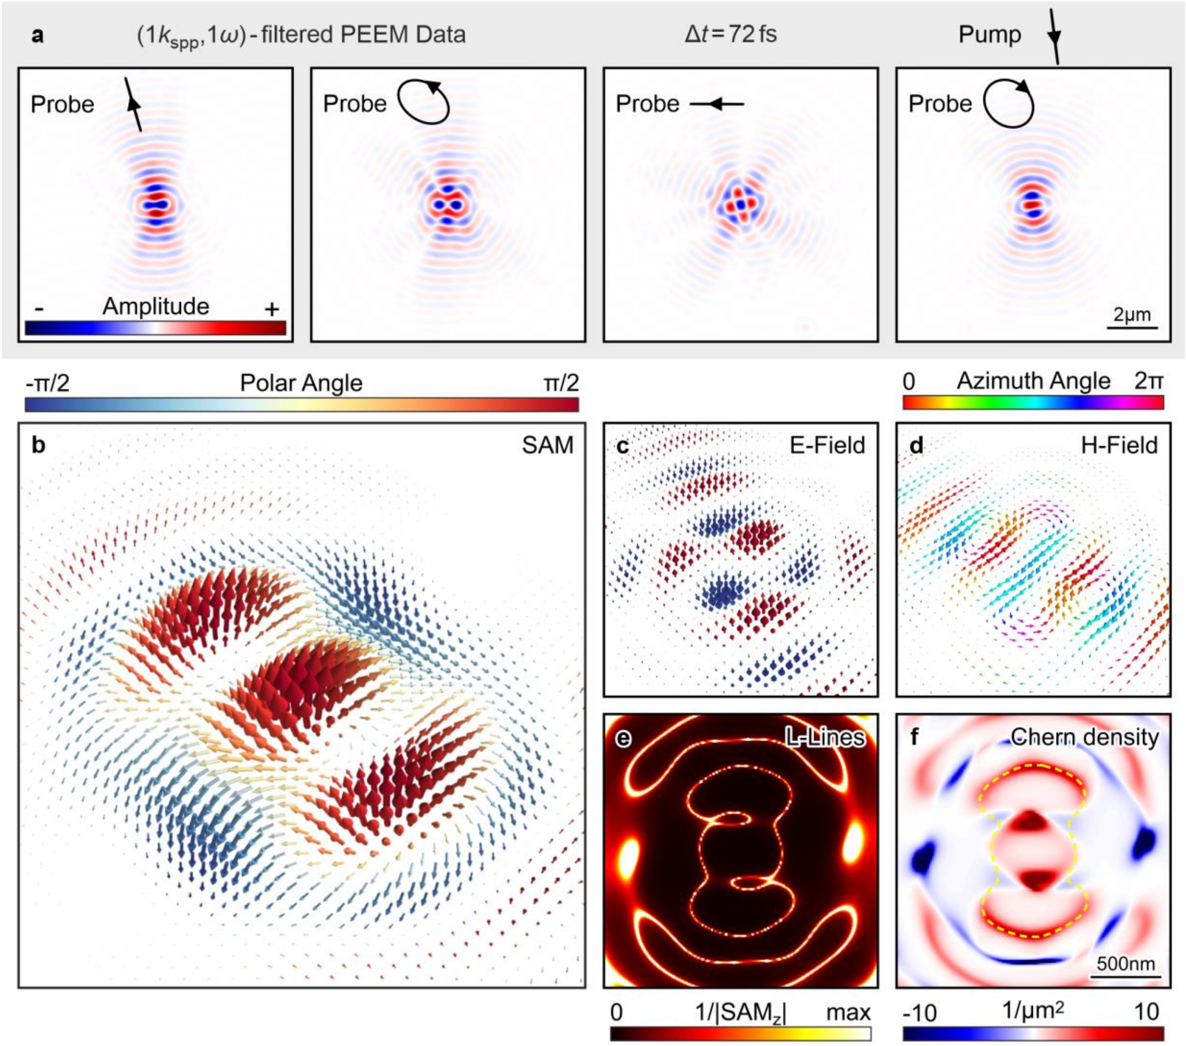


**Supplementary Figure 5:** Time-resolved polarimetric PEEM measurement of a trimeron at 72 fs delay time. (a) Fourier-filtered PEEM images for the same pump-, but different probe polarizations. (b) vector plot of the experimental SAM of the trimeron. The three (red) maxima each represent one meron. (c) electric field vectors of the trimeron as reconstructed from the PEEM measurements. (d) plot of the magnetic field vectors as calculated from the experimentally determined electric field vectors. (e) L-line singularity map from the experimental data. (f) Chern density as calculated from the experimental SAM with indicated integration region (dashed yellow line).

Supplementary Figure 5 summarizes the experimental data and results from our analysis. In analogy to Supplementary Figure 3b, Supplementary Fig. 5a shows the real part of Fourier-filtered pump-probe images for four different probe polarizations at a delay time of $\Delta t = 72$ fs. Supplementary Figure 5c shows the reconstructed electric field vectors. Blue arrows point into the surface and the red arrows point away from the surface. The corresponding $\mathbf{H}$-field is plotted in Supplementary Fig. 5d. The $\mathbf{H}$ field

lies entirely within the surface plane, as expected for the $\mathbf{H}$ field of an SPP. From both $\mathbf{E}$ and $\mathbf{H}$ field follows the SAM, which is plotted in Supplementary Fig. 5b. The time evolution of the experimentally determined SAM vectors is shown in Supplementary Video S1. It is noteworthy that the SAM texture is consistent with the theoretical prediction from Dai et al. [7]. The three broad (red) maxima each represent a SAM texture that consists of SAM vectors pointing out of the surface plane. The three maxima are surrounded by spin vectors pointing into the surface plane (blue). The bright lines in Supplementary Fig. 5e separate the two areas and indicate the locations where the transverse component of the SAM vectors crosses zero (L-lines). The trimeron in the center of the image is thus surrounded by a dumbbell-shaped L-line.

Note that Supplementary Fig. 5e can be directly compared to Figure 4d in supplementary Ref. [7], which was extracted with an optical-flow algorithm from a time-resolved PEEM experiment on a similar excitation structure and under comparable excitation conditions. The tremendous detail in the L-line topology in Fig. 5e demonstrates the quality of the data obtained with our new polarimetric PEEM method. It is important to note that in an analytical calculation of the SAM texture of the trimeron the shape of the innermost L-line is expected to exhibit a simple dumbbell-shape. The deviation from this expected shape in Fig. 5e is due to the pulsed nature of the excitation with femtosecond laser pulses. Our experimental data is almost identical to the results from the Finite Difference Time Domain simulation in Supplementary Video 3 in the work by Dai et al. [7]. Our own numerical simulations with a simple Hankel-wavelet model [9] also reproduce the exact L-line contour of Fig. 5e.

Supplementary Figure 5f shows the Chern density that was calculated from the SAM texture at a pump-probe delay of 72 fs. Numerically integrating over the outer contour of the dumbbell L-line in Fig. 5e (see dashed yellow line for the integration region) yields an overall Chern number of C=1.52, consistent with the expectation of C=3/2 for a trimeron.

**Supplementary Note 6:** Influence of the resolution on the Chern number

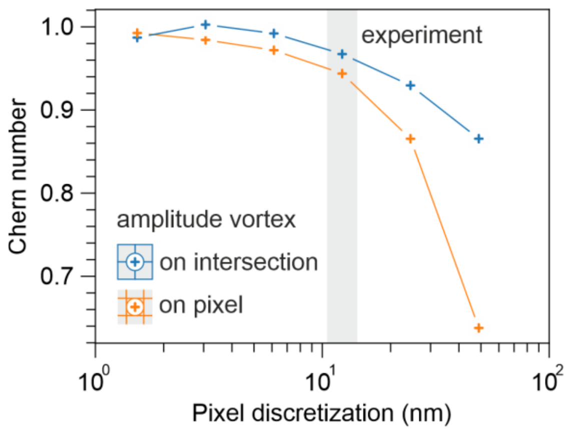


**Supplementary Figure 6:** Calculated Chern numbers from numerical simulations as function of pixel discretization. Results for two relative alignments of the amplitude vortex to the pixel grid are shown. The amplitude vortex can either be located on the pixel intersection (blue crosses) or the amplitude vortex can be centered on a pixel (orange crosses).

In the main manuscript the experimentally determined Chern number of the meron pair is slightly smaller than one, the expectation from an analytical solution. The deviation does not reflect a statistical inaccuracy of the measurement but is caused by the limited resolution of the discretization of the data by the detector, and by the exact position of the amplitude vortex between the two C-points of the meron pair relative to the detector pixel grid.

To support this statement, we performed numerical simulations of the SAM field for different pixel discretization and relative alignments of the meron SAM texture on a fictitious detector. The results are summarized in Supplementary Fig. 6, where the numerically integrated Chern number from simulated fields is plotted as function of the corresponding size of a detector pixel for the given field of view. As the discretization size increases, the calculated Chern number decreases, as the contribution of the (infinitely small) amplitude vortex to the Chern density becomes overestimated.

The second important contribution is the location of the amplitude vortex relative to the detector grid. If the amplitude vortex is located between pixels (blue crosses), it only partly contributes to the Chern number. If the amplitude vortex is located on a single pixel (orange crosses), it contributes more to the Chern Number.

From both contributions one would expect the estimated Chern number to decrease with increasing pixelation and that the on-pixel datapoints (orange crosses) have smaller Chern numbers. In the case of the real experiment, the calibrated field of view of 23.83 µm is imaged on a detector with 2048 × 2048 pixel, i.e. a corresponding pixel size of 12 nm, well-matched to the electron-optical resolution of the microscope of 10 nm. Our cross-correlation-based sub-pixel drift correction always puts the amplitude vortex right in the center of four pixels, and from Supplementary Fig. 6 we then expect a Chern number of 0.97, in excellent agreement to the average experimental Chern number (also C=0.97) in Fig. 4 of the main manuscript.

**Video Descriptions**

**Supplementary Video S1:** 3D View of the spin angular momentum of the trimeron that is discussed in Supplementary Note 5.

**Supplementary References**


[1] M. U. Wehner, M. H. Ulm, and M. Wegener, Optics Letters **22**, 1455 (1997).

[2] F. J. Meyer zu Heringdorf, D. Podbiel, N. Raß, A. Makris, N. M. Buckanie, and P. A. Kahl, Proc. SPIE **9921**, 992110 (2016).

[3] T. J. Davis, D. Janoschka, P. Dreher, B. Frank, F.-J. Meyer zu Heringdorf, and H. Giessen, Science **368**, 386 (2020).

[4] J. S. Li, L. Y. Zhong, S. D. Liu, Y. F. Zhou, J. Xu, J. D. Tian, and X. X. Lu, Sci Rep-Uk **7** (2017).

[5] A. Kubo, N. Pontius, and H. Petek, Nano Lett **7**, 470 (2007).

[6] P. Dreher, D. Janoschka, H. Giessen, R. Schützhold, T. J. Davis, M. Horn-von Hoegen, and F.-J. Meyer zu Heringdorf, Nanophotonics **13**, 1593 (2024).

[7] Y. A. Dai, Z. K. Zhou, A. Ghosh, R. S. K. Mong, A. Kubo, C. B. Huang, and H. Petek, Nature **588**, 616 (2020).

[8] D. Podbiel, P. Kahl, A. Makris, B. Frank, S. Sindermann, T. J. Davis, H. Giessen, M. Horn-von Hoegen, and F.-J. Meyer zu Heringdorf, Nano Letters **17**, 6569 (2017).

[9] T. J. Davis, B. Frank, D. Podbiel, P. Kahl, F.-J. Meyer zu Heringdorf, and H. Giessen, ACS Photonics **4**, 2461 (2017).
